# Supplementary material for: Correlations and Work Statistics in Critical Quantum Systems
Source: arXiv:2203.15464 source file (2022-03-29)
Supplement: Supplementary file 1 [file Appendix.tex]

\chapter{Other Information}
